# Supplementary material for: Cost-sensitive Learning for Utility Optimization in Online Advertising Auctions
Source: arXiv:1603.03713 source file (2017-07-12)
Supplement: Supplementary file 1 [file appendix.tex]

\appendix

\section{Extension to the probability of conversion}
\label{sec:extension}

So we far we have considered the case of a single model that tries to predict the probability of conversion given a display.
And in post-click attribution model the aim is more precisely to predict the probability of {\em post-click} conversions:
$$\Pr( \text{conversion}, \text{click} \mid \text{display}).$$

And it is possible to split that probability into the product of a click probability and a probability of conversion given click:
$$\Pr(\text{click} \mid \text{display}) \times \Pr( \text{conversion} \mid \text{click}).$$ 

Predicting these two probabilities independently offer two advantages: first it reduces the load on the data processing pipeline as there is no need to join impressions and conversions over a long period of time; and second it may predict more accurately campaigns with few or no conversions and a reasonable amount of clicks because in that case the clicks still provide some information on the effectiveness of the campaign.

Let us assume that the click model is already trained and that we want to train the second model, $\Pr( \text{conversion} \mid \text{click})$, with logistic regression. What should be be the weighting function used while training that model?

We will follow a similar approach as in Section 2: find the weighting such as to match the gradients of the log loss and the Utility loss.

The bid is now $p^c\times p\times v$ where $p^c$ is the already computed probability of click.
And the gradient is:
$$\frac{\partial \ell}{\partial p} \propto v^2p^c(p^c p-y) \times \frac{1}{p^c p v} = \frac{v(p^c p-y)}{p}$$
For a positive example this is approximatively $-v/p$ since $p_c p \ll 1$ and for a negative example this is $v p^c$.

We can not readily match the gradients since the Utility is computed on all the impressions while the conversion model is trained on the clicked impressions only.
\begin{eqnarray*} 
\mathbb{E}_{X,Y,C} f(X,Y) \mathbb{I}(C=1) & = & \mathbb{E}_{X,Y} \mathbb{E}_{C\mid X,Y} f(X,Y) \mathbb{I}(C=1) \\
& = & \mathbb{E}_{X,Y} \Pr(C = 1 \mid X,Y) f(X,Y)
\end{eqnarray*}

Replacing by the empirical distribution on both sides:
$$\mathbb{E} \sum_{i,~c_i=1} f(x_i, y_i) = \mathbb{E} \sum_i \Pr(C = 1 \mid X=x_i, Y=y_i) f(x_i, y_i)$$

Now let $f$ be the gradient of the log loss multiplied by the value $v_i$ of the conversion: $f(x_i, y_i) = [-y_i / p_i + (1-y_i) / (1-p_i)] v_i x_i$ with $p_i$ the predicted probability of conversion given click on $x_i$.

As in section 2, let us differentiate on the value of the label $y_i$.
\begin{enumerate}
\item $y_i=1$. \\
In this case $\Pr(C = 1 \mid x_i, Y = 1) = 1$ since by definition a post-click conversion is preceded with a click. 
The gradient on these examples is $-\sum_i v_i/p_i x_i$ which is close to the gradient of the Utility loss.
\item $y_i=0$. \\
We have $\Pr(C = 1 \mid x_i, Y = 0)$
\begin{eqnarray*}
%\Pr(C = 1 \mid x_i, Y = 0) & \\
& = & \frac{\Pr(Y=0 \mid x_i, C=1) \Pr(C=1 \mid x_i)}{\Pr(Y=0 \mid x_i)} \\
& \approx  & \Pr(C=1 \mid x_i) =  p^c_i
\end{eqnarray*}
The approximation relies on the assumption that the probabilities of conversion (given impression and given click) are small. 
And the gradient on these examples is about $\sum v_i p^c_i x_i$, same as for the Utility loss. 
\end{enumerate}
